# Supplementary material for: Utilizing Free Clients in Federated Learning for Focused Model Enhancement
Source: arXiv:2310.04515 source file (2023-10-06)
Supplement: Supplementary file 1 [file appendix.tex]

What are we gonna include in appendix
\begin{enumerate}
    \item Theorem for partial participation (imp), fedprox (Yes)
    \item Many other parameter values for number of internal vs external (Yes)
    \item Shakespeare
    \item Local model vs global model (Yes, but only in select cases)
\end{enumerate}
